# Supplementary material for: MLLM-Tool: A Multimodal Large Language Model For Tool Agent Learning
Source: arXiv:2401.10727 source file (2025-04-11)
Supplement: Supplementary file 2 [file hyperparameters.tex]

\begin{table}[!htb]
    \begin{center}
        \centering
        \resizebox{\linewidth}{!}{
        \begin{tabular}{c|c}
            Config  \\
            \midrule
            % Vision encoder &  \multicolumn{4}{c}{ViT-Huge} \\
            % embedding dim. & 768 & 384 & 768 & 512 \\
            % number of heads & 12 & 8 & 12 & 8 \\
            % number of layers & 12 & 12 & 12 & 6 \\
            Optimizer & AdamW \\
            Optimizer Momentum & $\beta_1=0.9, \beta_2=0.95$ \\
            Peak learning rate & 5e-4\\
            Weight decay & 0.001\\
            Warmup steps & 10 \\
            % Warmup epochs & \multicolumn{4}{c}{2} \\
            % Sample replication & 1.25 & 50 & 25 & 1.0 \\
            % Total epochs & 64 & 64 & 64 & 8 \\
            Batch size & 64\\
            Micro-batch size & 4\\
            Gradient accumulation steps & 4\\
            Maximum target length & 1024 \\
            % Batch size(13B) & 32\\
            % Micro-batch size(13B) & 1\\
            % Gradient accumulation steps(13B) & 8\\
            ImageBind Checkpoint & ImageBind-Huge \\
            \hline
            LoRA attention dimension (r) & 32\\
            LoRA scaling alpha ($\alpha$) & 32 \\
            LoRA drop out & 0.1
        \end{tabular}}
    \end{center}
    \caption{7B model training configuration.}
    \label{tab:pretrain_settings}
    \end{table}
