# Supplementary material for: MLLM-Tool: A Multimodal Large Language Model For Tool Agent Learning
Source: arXiv:2401.10727 source file (2025-04-11)
Supplement: Supplementary file 3 [file one2mul.tex]

\begin{table}[t!]
\small
  \centering
  
  \resizebox{\linewidth}{!}
  {
    \begin{tabular}{ccccc}
    \hline
    \multirow{2}{*}{Model} & \multicolumn{2}{c}{one-to-one} & \multicolumn{2}{c}{one-to-many}\\
\cmidrule(lr){2-3} \cmidrule(lr){4-5}          & Acc$\uparrow$ & \multicolumn{1}{c}{Hallu$\downarrow$} & Acc$\uparrow$ & Hallu$\downarrow$\\
    \hline

    Vicuna-7B (3epochs) & 51.75  & 6.71  & 86.62 & 1.23  \\
    Llama-7B (3epochs) & 56.12  & 6.85  & 85.86  & 3.04  \\
    Llama2-7B (3epochs) & 47.67  & 6.56  & 85.91  & 1.81  \\
    Llama2-Chat-7B (3epochs) & 57.29  & 6.56  & 83.75  & 4.27 \\
    \hline
    
    Vicuna-7B (5epochs) & 66.03  & 3.35  & 90.01  & 0.94  \\
    Llama-7B (5epochs) & {69.24}  & 1.31  & 90.59 & 0.29  \\
    Llama2-7B (5epochs) & 63.12  & 3.64  & 87.73  & 1.29  \\
    Llama2-Chat-7B (5epochs) & 70.99 & 2.33  & 88.66  & 0.94  \\
    \hline
    Vicuna-13B (3epochs) & 47.96  & 7.14  & 86.09  & 1.64  \\
    Llama-13B (3epochs) & 47.23  & 5.69  & 85.21  & 2.81  \\
    Llama2-13B (3epochs) & 51.90  & 8.16  & 87.78  & 1.46  \\
    Llama2-Chat-13B (3epochs) & 41.84  & 7.00  & 73.87  & 1.93 \\
    \hline
    Vicuna-13B (5epochs) & 61.95  & 4.52  & 89.25  & 0.99 \\
    Llama-13B (5epochs) & 61.81  & 3.35  & 88.49  & 0.94  \\
    Llama2-13B (5epochs) & 62.97  & 3.06  & 88.72  & 0.76  \\
    Llama2-Chat-13B (5epochs) & 50.58  & 3.35  & 74.40  & 0.53  \\
    \hline
    
    Vicuna-13B (10epochs) & \textbf{77.26}  & 0.58  & \textbf{92.58}  & 0.00 \\
    Llama-13B (10epochs) & \uline{76.68}  & 0.58  & \uline{92.34}  & 0.00  \\
    Llama2-13B (10epochs) & 69.24  & 0.44  & 86.85  & 0.06  \\
    Llama2-Chat-13B (10epochs) & 76.38  & 0.29  & \uline{92.34}  & 0.00 \\
    \hline
    
    \end{tabular}}%
  \caption{The performance on testing subsets divided by API option number.}
    \label{tab:suppl_one2mul}%
\end{table}%
