# Supplementary material for: MLLM-Tool: A Multimodal Large Language Model For Tool Agent Learning
Source: arXiv:2401.10727 source file (2025-04-11)
Supplement: Supplementary file 4 [file recall.tex]

% Table generated by Excel2LaTeX from sheet 'all'
\begin{table}[htbp]
  \centering
    \begin{tabular}{cc}
    \hline
    Model & Recall$\uparrow$ \\
    \hline
    Llama2-7B  & \textbf{62.13} \\
    Llama2-Chat-7B & \uline{61.47} \\
    \hline
    \end{tabular}%
  \caption{The recall performance of two 7B models.}
\label{tab:1}%
\end{table}%
